# Supplementary material for: Morpheus: Text-Driven 3D Gaussian Splat Shape and Color Stylization
Source: arXiv:2503.02009 source file (2025-03-18)
Supplement: Supplementary file 1 [file comparisons_transposed_supp_3.tex]

\setlength\tabcolsep{0pt}

\begin{tabular}{ccccccc}
    \centering

     & Original & GaussCtrl~\cite{wu2024gaussctrl} & Instruct-GS2GS~\cite{vachha2024instruct} & Instruct-N2N~\cite{haque2023instruct} & DGE~\cite{chen2024dge} & Ours \\

    \raisebox{1.0\height}{\parbox[t]{12mm}{\rotatebox[origin=c]{90}{\makecell{a photo of a \\ Batmobile}}}}
    & \includegraphics[width=0.151\textwidth]{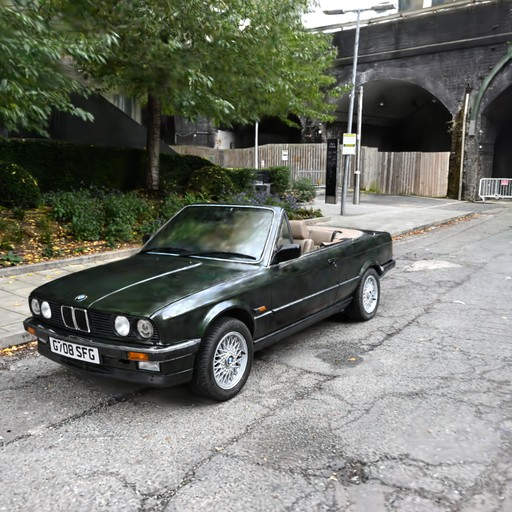}
    & \includegraphics[width=0.151\textwidth]{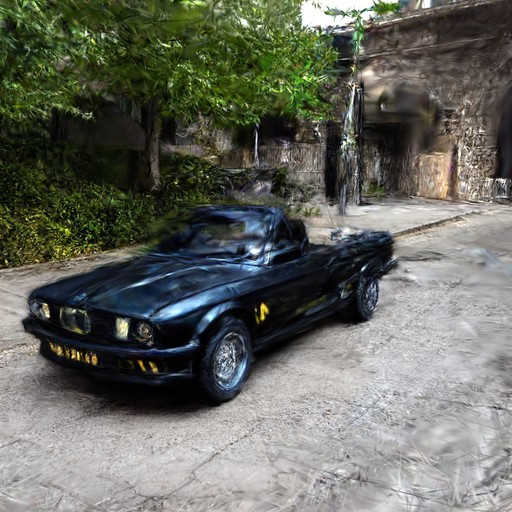}
    & \includegraphics[width=0.151\textwidth]{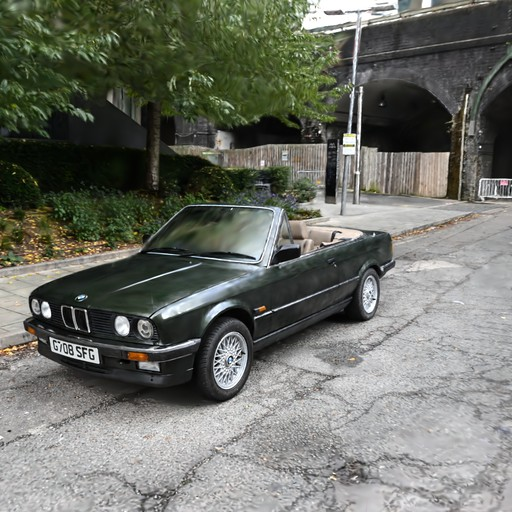}
    & \includegraphics[width=0.151\textwidth]{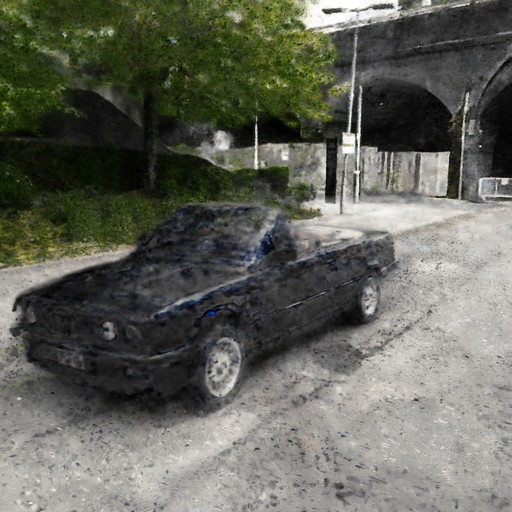}
    & \includegraphics[width=0.151\textwidth]{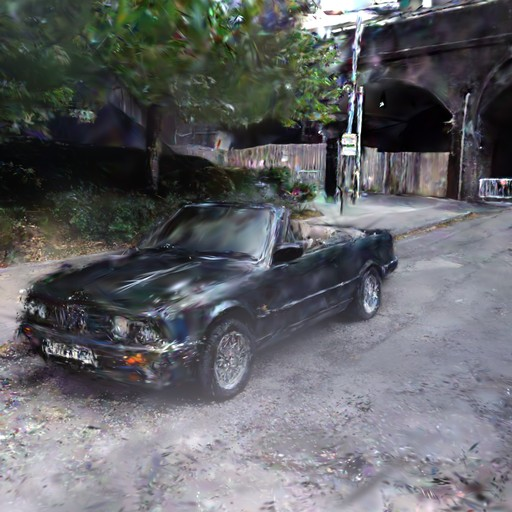}
    & \includegraphics[width=0.151\textwidth]{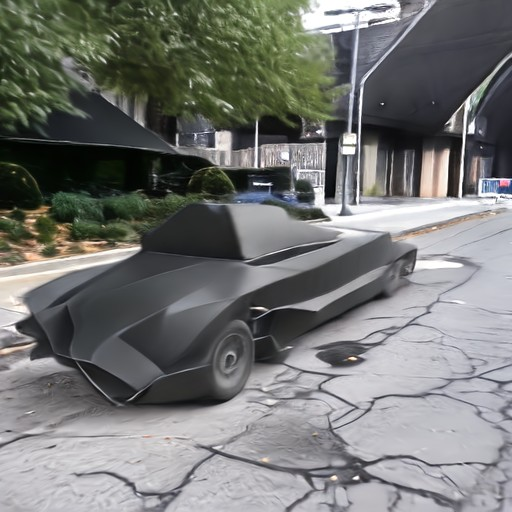}
    \\

    \raisebox{1.0\height}{\parbox[t]{12mm}{\rotatebox[origin=c]{90}{\makecell{a screenshot of \\ a Minecraft car}}}}
    & \includegraphics[width=0.151\textwidth]{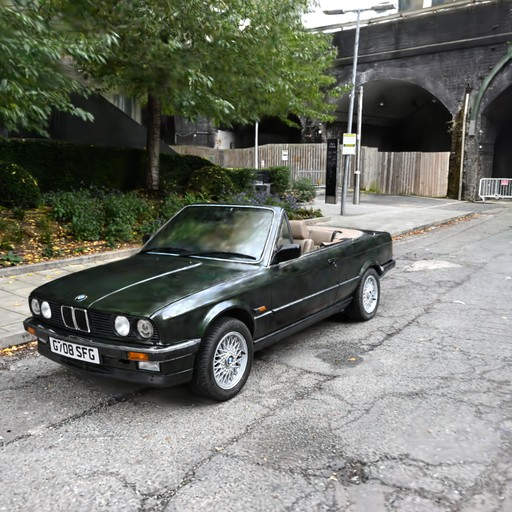}
    & \includegraphics[width=0.151\textwidth]{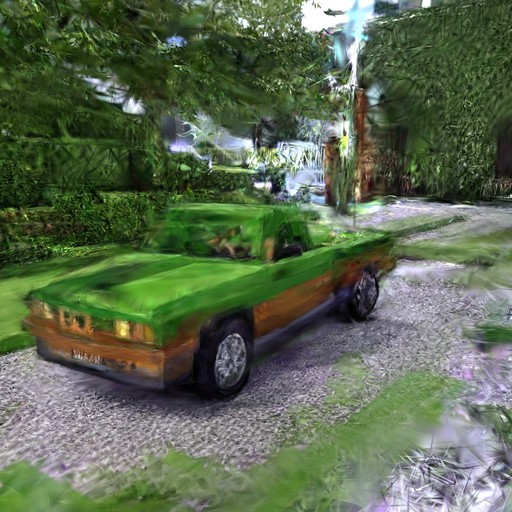}
    & \includegraphics[width=0.151\textwidth]{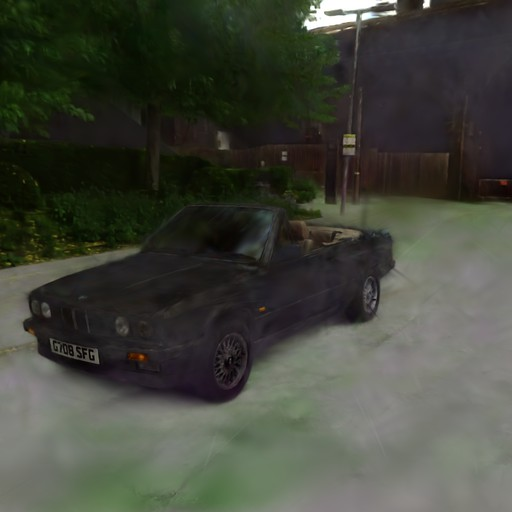}
    & \includegraphics[width=0.151\textwidth]{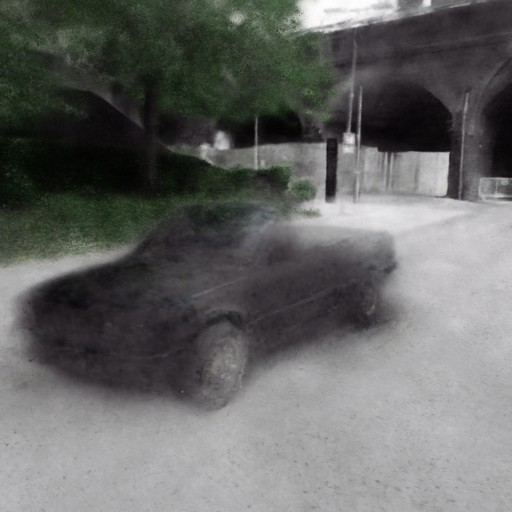}
    & \includegraphics[width=0.151\textwidth]{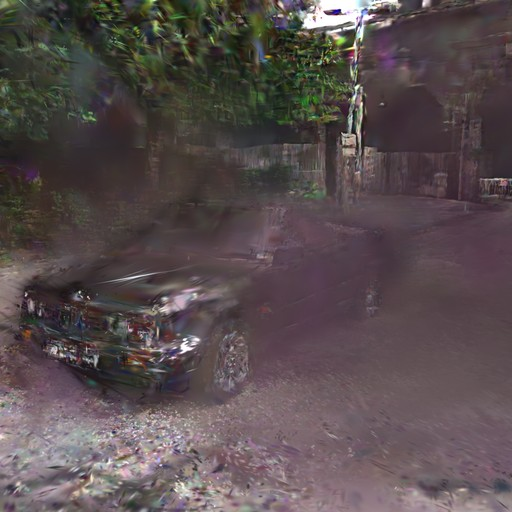}
    & \includegraphics[width=0.151\textwidth]{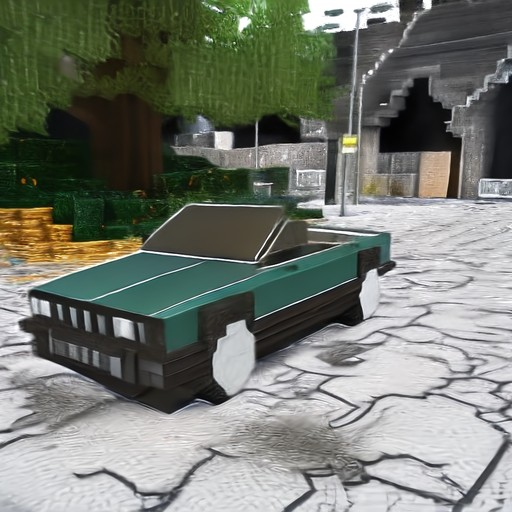}
    \\

    \raisebox{1.0\height}{\parbox[t]{12mm}{\rotatebox[origin=c]{90}{\makecell{Modern art \\ studio with \\ paint \\ splatters, \\ canvases, and \\ abstract \\ sculptures}}}}
    & \includegraphics[width=0.151\textwidth]{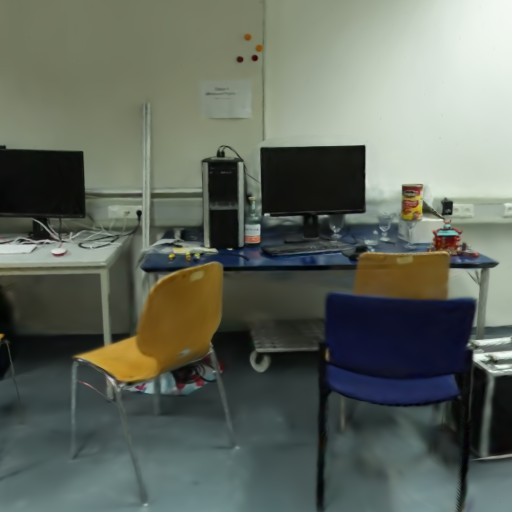}
    & \includegraphics[width=0.151\textwidth]{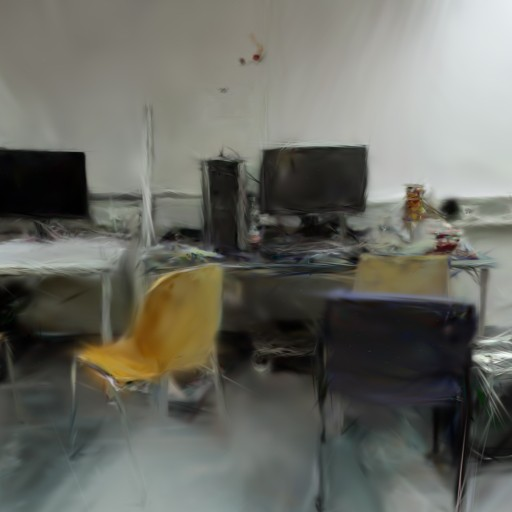}
    & \includegraphics[width=0.151\textwidth]{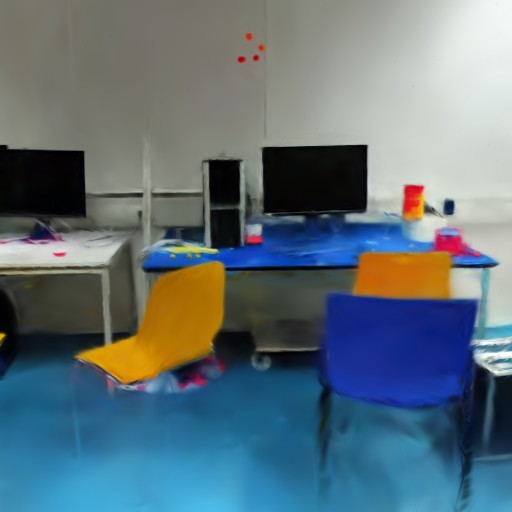}
    & \includegraphics[width=0.151\textwidth]{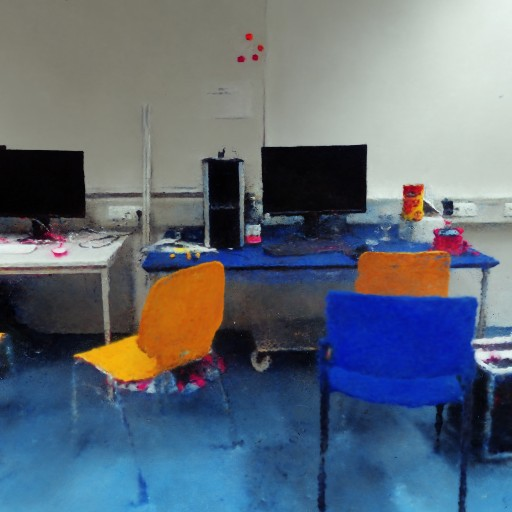}
    & \includegraphics[width=0.151\textwidth]{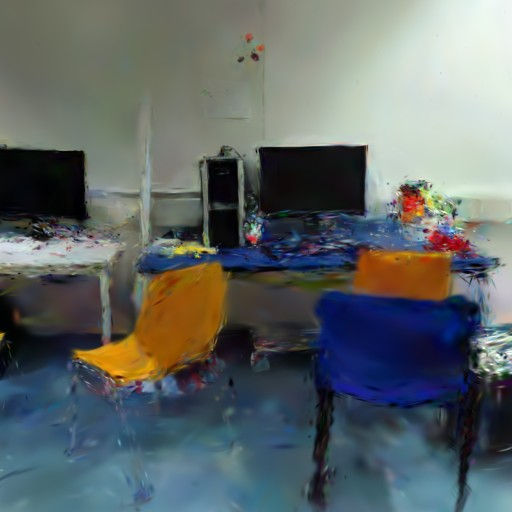}
    & \includegraphics[width=0.151\textwidth]{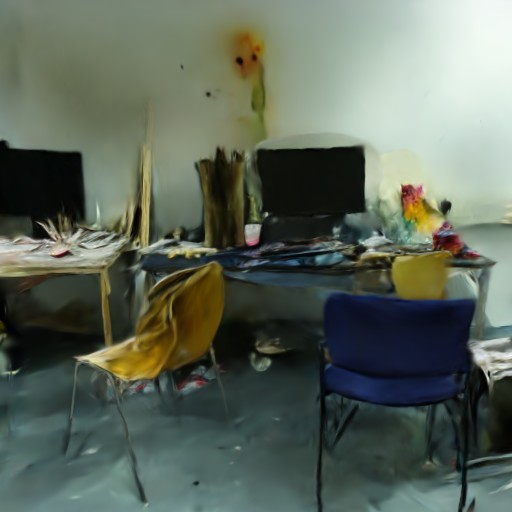}
    \\

    \raisebox{1.0\height}{\parbox[t]{12mm}{\rotatebox[origin=c]{90}{\makecell{a Fauvism \\ painting of a \\ photo of a \\ conference room \\ with tables and \\ chairs}}}}
    & \includegraphics[width=0.151\textwidth]{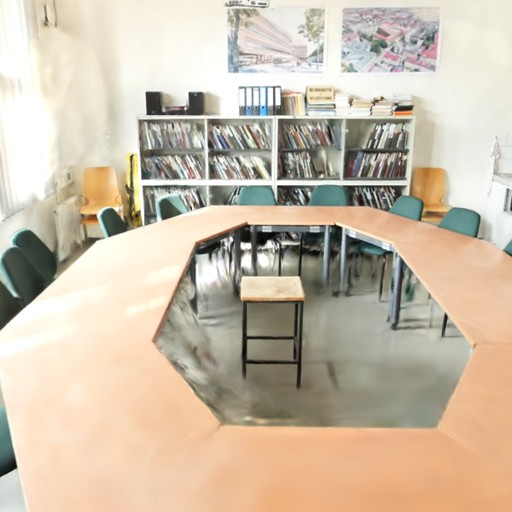}
    & \includegraphics[width=0.151\textwidth]{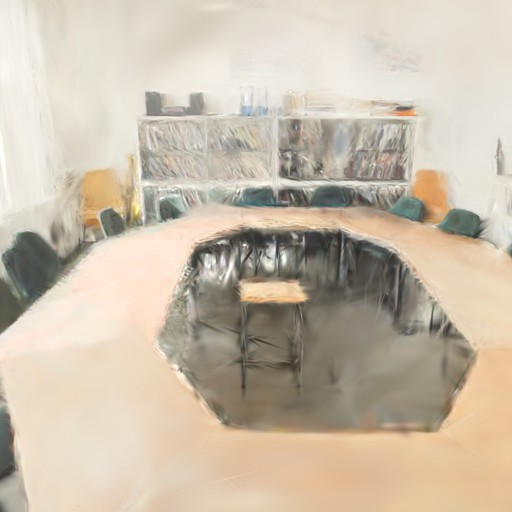}
    & \includegraphics[width=0.151\textwidth]{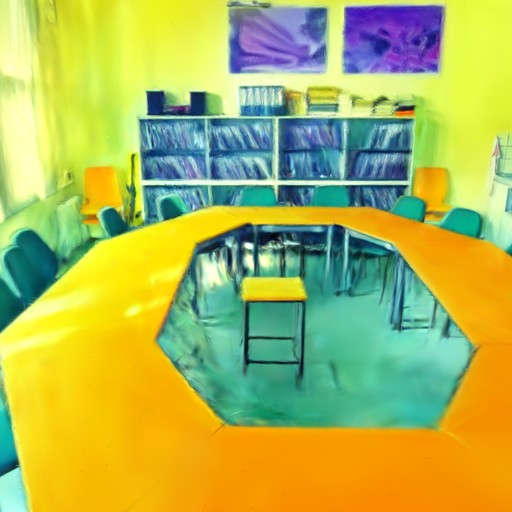}
    & \includegraphics[width=0.151\textwidth]{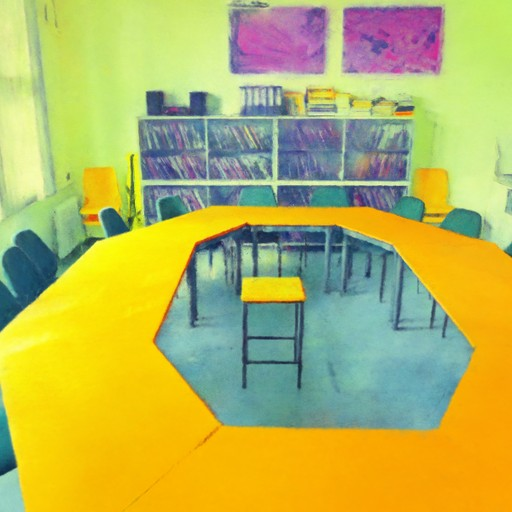}
    & \includegraphics[width=0.151\textwidth]{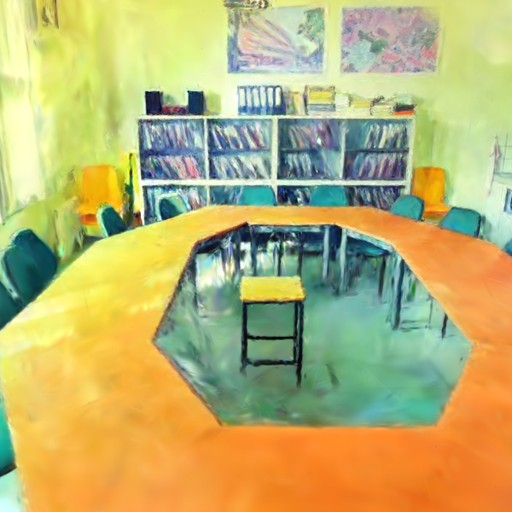}
    & \includegraphics[width=0.151\textwidth]{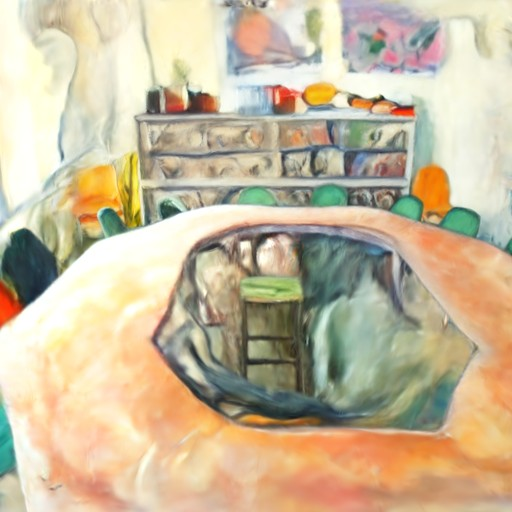}
    \\

    \raisebox{1.0\height}{\parbox[t]{12mm}{\rotatebox[origin=c]{90}{\makecell{a Hiroshige \\ Utagawa \\ painting of a \\ kitchen}}}}
    & \includegraphics[width=0.151\textwidth]{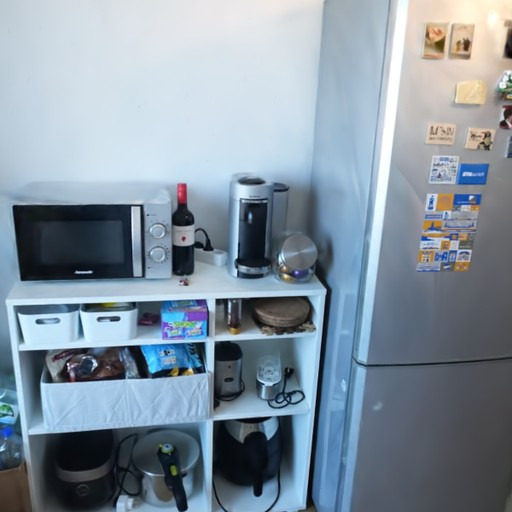}
    & \includegraphics[width=0.151\textwidth]{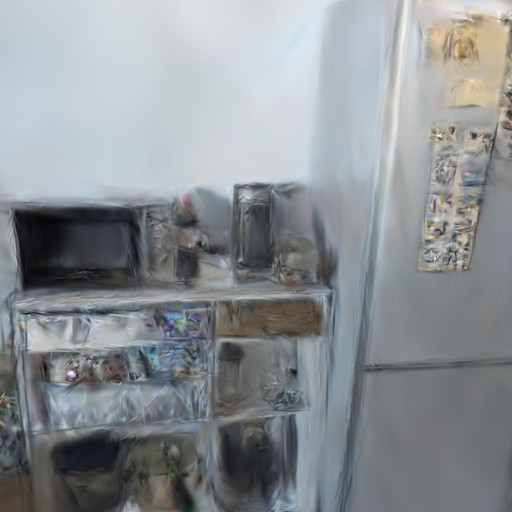}
    & \includegraphics[width=0.151\textwidth]{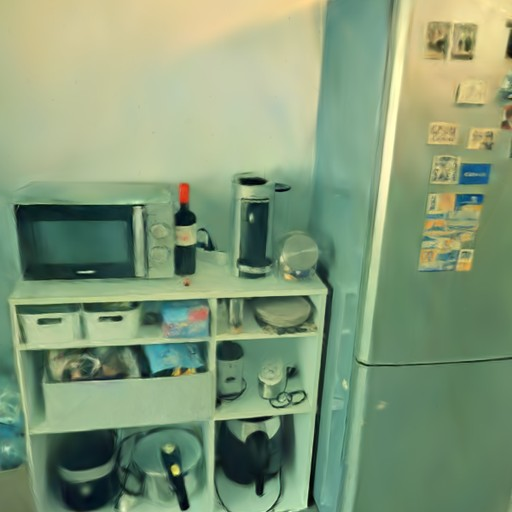}
    & \includegraphics[width=0.151\textwidth]{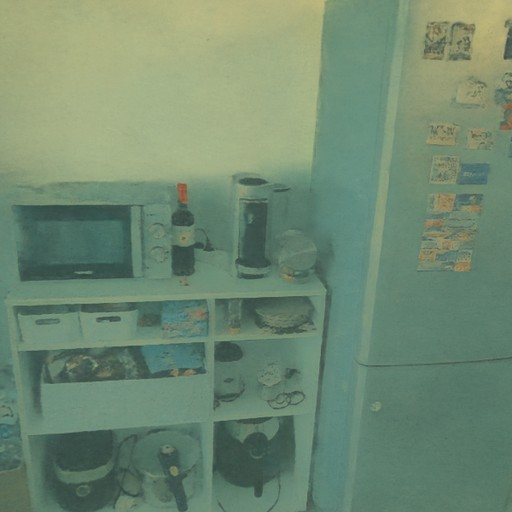}
    & \includegraphics[width=0.151\textwidth]{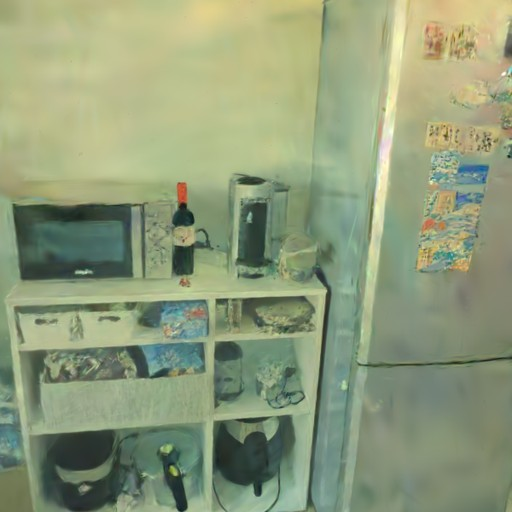}
    & \includegraphics[width=0.151\textwidth]{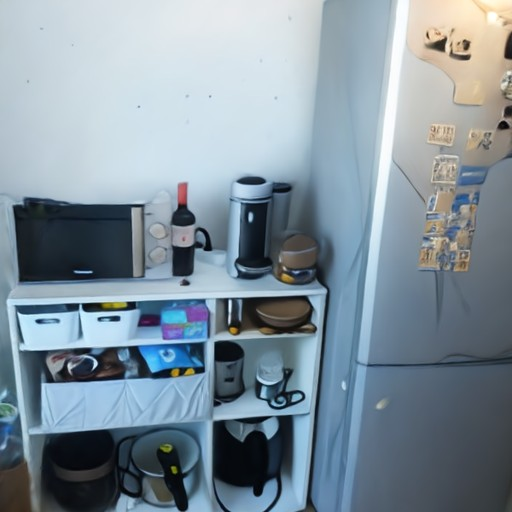}
    \\

    \raisebox{1.0\height}{\parbox[t]{12mm}{\rotatebox[origin=c]{90}{\makecell{a Bastion game \\ style picture \\ of a flat with \\ a bathroom, \\ living room and \\ a kitchen}}}}
    & \includegraphics[width=0.151\textwidth]{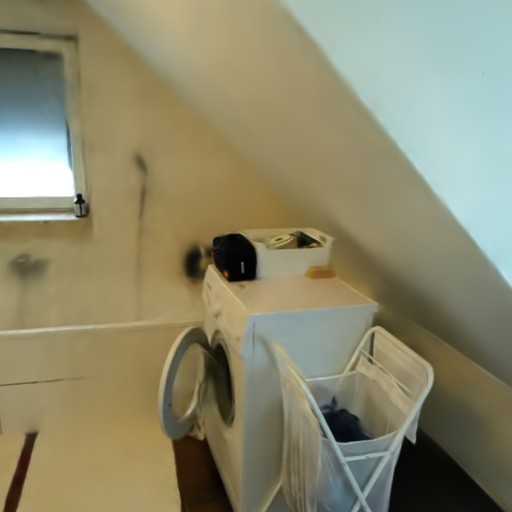}
    & \includegraphics[width=0.151\textwidth]{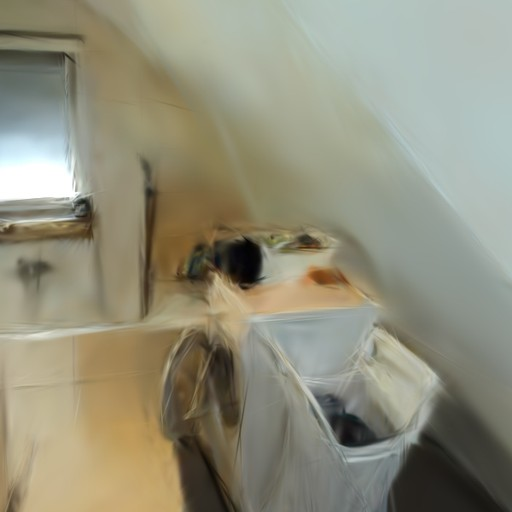}
    & \includegraphics[width=0.151\textwidth]{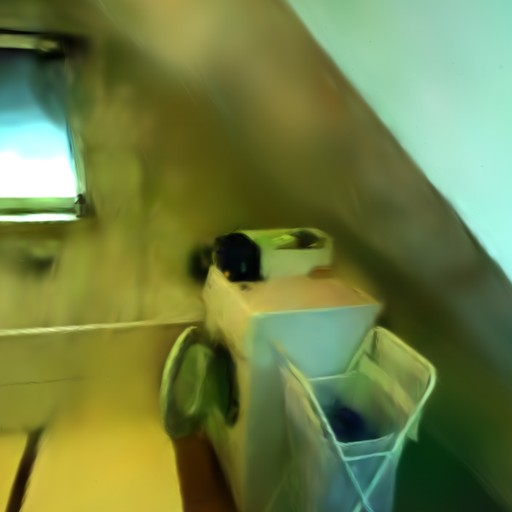}
    & \includegraphics[width=0.151\textwidth]{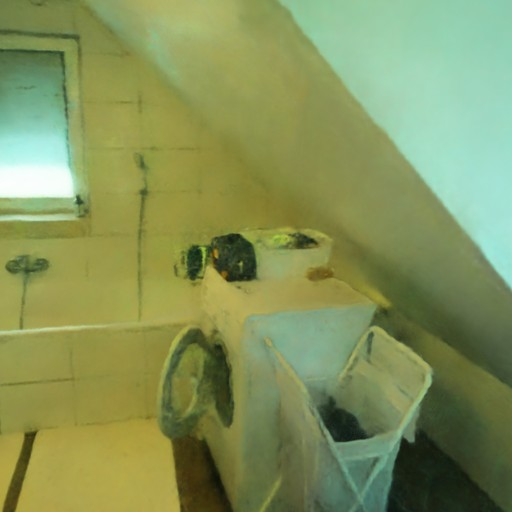}
    & \includegraphics[width=0.151\textwidth]{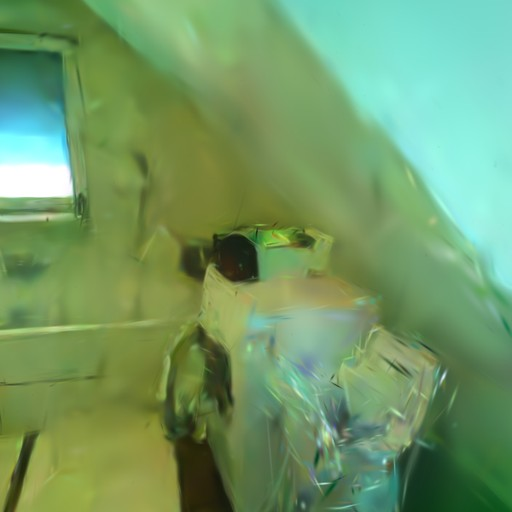}
    & \includegraphics[width=0.151\textwidth]{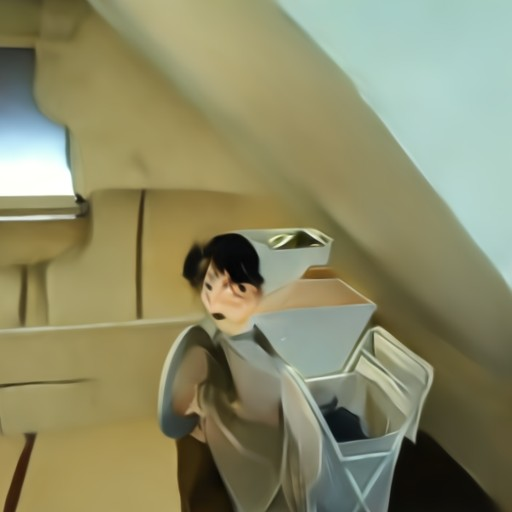}
    \\

\end{tabular}
